# Supplementary material for: Enabling Autoregressive Models to Fill In Masked Tokens
Source: arXiv:2502.06901 source file (2025-02-09)
Supplement: Supplementary file 1 [file appendix.tex]

\newpage
\appendix
\onecolumn
\section{You \emph{can} have an appendix here.}
